# Supplementary material for: Topological Polaritons
Source: arXiv:1406.4156 source file (2015-06-17)
Supplement: Supplementary file 1 [file topolaritons_supp_mat.pdf]

# Supplemental Material for "Topological polaritons"

Torsten Karzig,[1] Charles-Edouard Bardyn,[1] Netanel Lindner,[2,1] and Gil Refael[1]

[1]*Institute for Quantum Information and Matter, Caltech, Pasadena, California 91125, USA*
[2]*Physics Department, Technion, 32000 Haifa, Israel*

## I. EXCITON-PHOTON COUPLING INCLUDING TE AND TM MODES

In this section, we complement the discussion of the exciton/TE-photon coupling of the main text by including the effect of the TM mode. This is especially relevant for small momenta where the TE and TM modes become degenerate, and clarifies the meaning of the apparent non-analyticity of the exciton/TE-photon coupling $\sim \exp(\mathrm{i}\theta_q)$ for $q \to 0$.

### A. Electron-photon coupling

Following along the lines of the main text, we start from a quantum well described by the Hamiltonian

$$H_{\mathrm{QW}}(\mathbf{k}) = \left[M + B\left(k_x^2 + k_y^2\right)\right]\sigma_z + A\left(k_x\sigma_x + k_y\sigma_y\right), \tag{1}$$

selected over its time-reversed counterpart by an external magnetic field. In this case the corresponding excitons have total angular momentum $J_z = +1$. (We discuss numerics including both $J_z = \pm 1$ excitons further below.) For a large exciton Bohr radius $a_0 \gg A/M$, we can work in the low-momentum regime and the leading exciton-photon coupling takes the form

$$H_{\mathrm{ex-ph}} = \sqrt{\frac{2}{\pi}}\frac{A}{a_0}\sum_{\mathbf{q}} \hat{b}_{\mathbf{q}}^\dagger \hat{\mathbf{A}}_q \cdot (\mathbf{e}_x - \mathrm{i}\mathbf{e}_y) + \mathrm{H.c.}, \tag{2}$$

in terms of the quantized vector potential $\hat{\mathbf{A}}_q$. As a minimal model of the cavity, we consider perfect metallic parallel-plate mirrors. The corresponding photonic modes are of TE and TM type,

$$\hat{\mathbf{A}}_q = F_q\left(\mathbf{e}_{\mathbf{q}\perp}\sin(q_d z)\hat{a}_q^{\mathrm{TE}} + \left[\sqrt{1-f_q^2}\mathbf{e}_{\mathbf{q}\parallel}\sin(q_d z) - \mathrm{i}f_q\mathbf{e}_z\cos(q_d z)\right]\hat{a}_q^{\mathrm{TM}}\right) + \mathrm{H.c.}(\mathbf{q}\to-\mathbf{q}), \tag{3}$$

where $\mathbf{e}_{q\parallel}$ and $\mathbf{e}_{q\perp}$ are in-plane unit vectors parallel and perpendicular to $\mathbf{q}$, $q_d = m\pi/d$ is the momentum of the $m$th standing wave in the $z$-direction of the cavity with height $d$, and $f_q = 1/\sqrt{1+(q_d/q)^2}$. In the following we assume that the quantum well is located in the anti-nodes of the in-plane electric field, such that $\sin(q_d z) = 1$. Using Eq. (2) and keeping only the resonant contributions, we then obtain

$$H_{\mathrm{ex-ph}} = \sqrt{\frac{2}{\pi}}\frac{A}{a_0}F_q\sum_{\mathbf{q}}\hat{b}_{\mathbf{q}}^\dagger\left(-\mathrm{i}\mathrm{e}^{-\mathrm{i}\theta_{\mathbf{q}}}\hat{a}_{\mathbf{q}}^{\mathrm{TE}} + \sqrt{1-f_q^2}\mathrm{e}^{-\mathrm{i}\theta_{\mathbf{q}}}\hat{a}_{\mathbf{q}}^{\mathrm{TM}}\right) + \mathrm{H.c.}, \tag{4}$$

which agrees in the $q \gg g_d$ limit ($f_{q\gg q_d} = 1$) with the TE-only coupling derived in the main text [cf. Eq. (8)]. In general, however, the exciton will couple to both modes with coupling strengths becoming equal for small momenta. This leads to a hybridization of the edge mode with the TM bulk modes. To study the low-momentum regime, it is convenient to switch to a basis of right- and left-handed circular polarizations via

$$\hat{a}_{\mathbf{q}}^{\mathrm{TE}} = \frac{\mathrm{i}}{\sqrt{2}}\left(\mathrm{e}^{\mathrm{i}\theta_{\mathbf{q}}}\hat{a}_{\mathbf{q}}^{+} - \mathrm{e}^{-\mathrm{i}\theta_{\mathbf{q}}}\hat{a}_{\mathbf{q}}^{-}\right) \tag{5}$$

$$\hat{a}_{\mathbf{q}}^{\mathrm{TM}} = \frac{1}{\sqrt{2}}\sqrt{1-f_q^2}\left(\mathrm{e}^{\mathrm{i}\theta_{\mathbf{q}}}\hat{a}_{\mathbf{q}}^{+} + \mathrm{e}^{-\mathrm{i}\theta_{\mathbf{q}}}\hat{a}_{\mathbf{q}}^{-}\right), \tag{6}$$

where operators $\hat{a}_{\mathbf{q}}^{\pm\dagger}$ create photonic modes with polarization vectors $\mathbf{e}_{\pm} = (1, \pm\mathrm{i})/\sqrt{2}$. The exciton-photon coupling then reads

$$H_{\mathrm{ex-ph}} = \sqrt{\frac{1}{\pi}}\frac{A}{a_0}F_q\sum_{\mathbf{q}}\hat{b}_{\mathbf{q}}^\dagger\left[(2-f_q^2)\hat{a}_{\mathbf{q}}^{+} - f_q^2\mathrm{e}^{-2\mathrm{i}\theta_{\mathbf{q}}}\hat{a}_{\mathbf{q}}^{-}\right] + \mathrm{H.c.}. \tag{7}$$

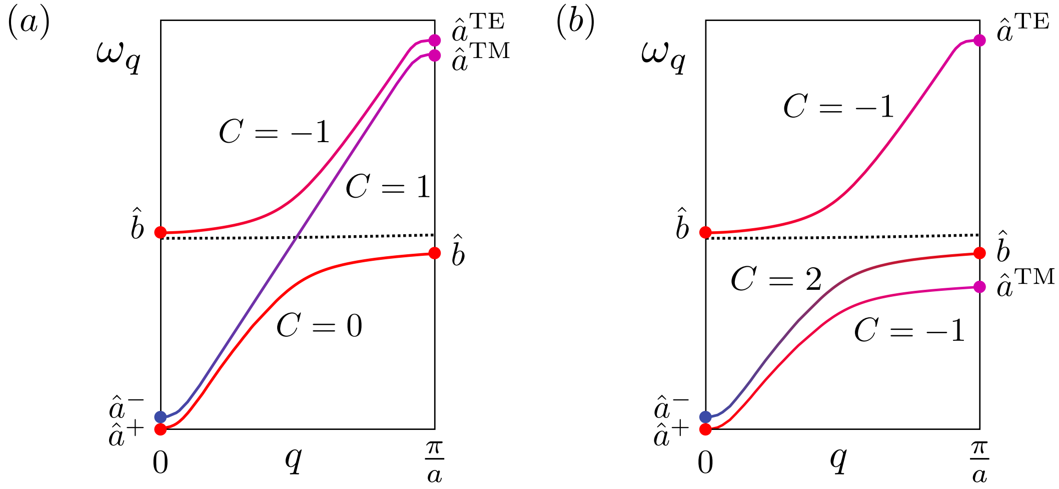


FIG. 1. Illustration of the polariton-band topology (as indicated by the corresponding Chern numbers $C$) for an exciton ($J_z = +1$) coupled to two photonic modes without (a) and with (b) strong TE/TM splitting. The polariton bands are drawn schematically in a (simplified) one-dimensional Brillouin zone created by an external periodic potential of period $a$. The backfolded bands from higher Brillouin zones are omitted for clarity. The color coding indicates the $J_z$ total angular momentum with red/purple/blue corresponding to $J_z = 1/0/-1$. The dashed black line shows the bare exciton band.

Note that using the static $\mathbf{e}_\pm$ instead of the polar $\mathbf{e}_{\mathbf{q}\|/\perp}$ basis removes all apparent non-analyticities at $q = 0$ in Eq. (7). For small momenta, the exciton couples with a constant coupling to the right-handed polarized mode, while the (double) winding coupling to the left-handed polarized mode vanishes as $(q_x - \mathrm{i}q_y)^2$. The winding in the coupling can be seen as a simple consequence of angular momentum conservation required when mixing the $J_z = +1$ exciton with the $J_z = \pm 1$ photons. Note that in the large-momentum regime the exciton couples to an equal superposition of circularly polarized modes $(\mathrm{e}^{\mathrm{i}\theta_\mathbf{q}}\hat{a}^+_\mathbf{q} - \mathrm{e}^{-\mathrm{i}\theta_\mathbf{q}}\hat{a}^-_\mathbf{q})$, which is exactly the TE mode. The single winding of the exciton/TE-photon coupling then results from $m_z^{TE} = 0$. We remark that there is a relation between the exciton/TE-photon coupling $g_\mathbf{q}$ and the low-momentum exciton/right-handed-polarized photon coupling $\Omega = \sqrt{4/\pi}AF_q/a_0$,

$$g_\mathbf{q} = -\mathrm{i}\frac{\Omega}{\sqrt{2}}\mathrm{e}^{-\mathrm{i}\theta_\mathbf{q}}\,, \tag{8}$$

which can be read off from Eqs. (4) and (7).

### B. Band topology

The full Hamiltonian of the system with two excitons ($J_z = \pm 1$) and two photons (right- and left-handed circularly polarized) takes the form

$$H = \sum_\mathbf{q} \begin{pmatrix} \hat{a}^{+\dagger}_\mathbf{q} & \hat{a}^{-\dagger}_\mathbf{q} & \hat{b}^{+\dagger}_\mathbf{q} & \hat{b}^{-\dagger}_\mathbf{q} \end{pmatrix} \begin{pmatrix} \omega^C(q) & \Delta^{\mathrm{LT}}(q)\mathrm{e}^{-2\mathrm{i}\theta_\mathbf{q}} & \frac{\Omega}{2}(2-f_q^2) & -\frac{\Omega}{2}f_q^2\mathrm{e}^{-2\mathrm{i}\theta_\mathbf{q}} \\ \Delta^{\mathrm{LT}}(q)\mathrm{e}^{2\mathrm{i}\theta_\mathbf{q}} & \omega^C(q) & -\frac{\Omega}{2}f_q^2\mathrm{e}^{2\mathrm{i}\theta_\mathbf{q}} & \frac{\Omega}{2}(2-f_q^2) \\ \frac{\Omega}{2}(2-f_q^2) & -\frac{\Omega}{2}f_q^2\mathrm{e}^{-2\mathrm{i}\theta_\mathbf{q}} & \omega^X(q)+\Delta_Z & 0 \\ -\frac{\Omega}{2}f_q^2\mathrm{e}^{2\mathrm{i}\theta_\mathbf{q}} & \frac{\Omega}{2}(2-f_q^2) & 0 & \omega^X(q)-\Delta_Z \end{pmatrix} \begin{pmatrix} \hat{a}^+_\mathbf{q} \\ \hat{a}^-_\mathbf{q} \\ \hat{b}^+_\mathbf{q} \\ \hat{b}^-_\mathbf{q} \end{pmatrix}$$
$$+ \sum_{\mathbf{q}\mathbf{q}'\tau=\pm} \hat{a}^{\tau\dagger}_{\mathbf{q}'}V^C(\mathbf{q}'-\mathbf{q})\hat{a}^\tau_\mathbf{q} + \hat{b}^{\tau\dagger}_{\mathbf{q}'}V^X(\mathbf{q}'-\mathbf{q})\hat{b}^\tau_\mathbf{q}\,, \tag{9}$$

where $\omega^{C(X)}(q)$ denotes the bare photon (exciton) dispersion, $\Delta_Z$ is the exciton Zeeman splitting, and $V^{C(X)}(\mathbf{q})$ is the Fourier transform of the periodic photon (exciton) potential. The coupling terms $\Delta^{\mathrm{LT}}(q)\mathrm{e}^{\pm 2\mathrm{i}\theta_\mathbf{q}}$ arise from a finite energy splitting between TE and TM modes. For small momenta, the energy shift of the TE(TM) photons takes the form $+(-)\Delta_{\mathrm{LT}}q^2$. Using Eqs. (5) and (6), one then finds $\Delta^{\mathrm{LT}}(q) = -\Delta_{\mathrm{LT}}q^2$, which we will use in the following.

To understand the topology emerging form the Hamiltonian (9), we first focus on the interplay of a single ($J_z = +1$) exciton with both photonic modes, as shown schematically in Fig. 1. At $q = 0$, the eigenmodes are of right- or left-handed-polarized nature, with the mode of $\hat{a}^+$ character at slightly lower energy due to the finite coupling to the

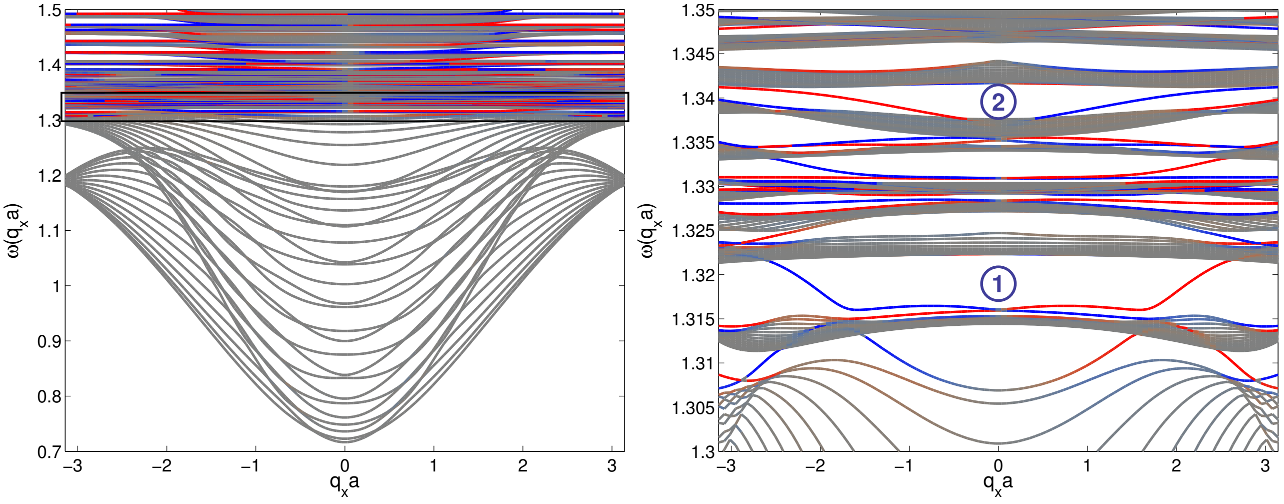


FIG. 2. Energy spectrum of Zeeman-split excitons coupled resonantly to TE photons, with gapped-out TM modes. The left panel shows an overview of the spectrum. We choose a triangular periodic exciton and photon potential where a finite linear-transverse splitting $\Delta_{LT} = 0.15$ allows for a gap in the TM modes clearly visible at energies above $\approx 1.2$. The remaining numerical parameters (setting the units as in the main text) are given by $c = 1$, $q_d = 1$, $\omega_0^X = 1.3$, $m_X = 10^5$, $\Delta_Z = 0.01$, $g = 0.1$, $a = 1.8$, $V_X = 0.05$ and $V_C = 0.6$. The right panel shows a zoom-in of the region close to the lowest-energy polariton (marked by a black rectangle in the left panel). The color encodes the edge localization of the modes with red(blue) indicating a large weight of the wavefunction at the edge at $y = 0 (y = L)$. Note that one observes topological gaps. The lowest gap of each edge-mode chirality is marked by an encircled number. The numbered gaps are separated by the Zeeman splitting $2\Delta_z$ and correspond to the time-reversed excitons with $J_z = -1$ (gap 1) and $J_z = +1$ (gap 2).

exciton. Assuming that the Brillouin-zone boundary (defined by the periodic potentials) is at momenta large compared to $q_d$, the states at the Brillouin-zone boundary have TE/TM character. Figure 1(a) shows the case of weak TE/TM splitting where the exciton is resonant with both the TE and the TM mode. While there are bands with non-trivial Chern numbers $C$, a topological gap can only be found in case of Fig. 1(b) where the exciton is resonant only with the TE mode while the TM mode is gapped.

As an example of a system with Hamiltonian (9) and a finite gap for TM modes, we consider a cavity/photonic crystal with a triangular photonic potential

$$V^C(x, y) = V_C \left[ \cos\left(\frac{4\pi}{\sqrt{3}a} y\right) + \cos\left(\frac{2\pi x}{a} + \frac{2\pi y}{\sqrt{3}a}\right) + \cos\left(\frac{2\pi x}{a} - \frac{2\pi y}{\sqrt{3}a}\right)\right], \tag{10}$$

to provide photonic gaps. The TE/TM splitting then shifts the energy of the TE and TM gap relative to each other, allowing for energies where only TE photons are present. To study the presence of edge modes, we calculate the band structure in a stripe geometry with periodic boundary conditions in $x$-direction, and vanishing boundary conditions in $y$-direction. Moreover, we use the photon and exciton dispersions $\omega^C(q) = c\sqrt{q^2 + q_d^2}$ and $\omega_\pm^X(q) = q^2/2m_X + \omega_0^X$, respectively. A finite exciton Zeeman splitting and periodic exciton potential of the form (10) with strength $V_X$ then allows to open up a topological gap. The resulting energy spectrum is depicted in Fig. 2 and shows a pair of topological gaps, corresponding to the Zeeman-split $J_z = \pm 1$ excitons. Since the respective exciton-photon couplings of the two excitons are related by time-reversal symmetry, the edge modes in each gap have opposite chirality.

## II. DRIVEN-DISSIPATIVE GROSS-PITAEVSKII EQUATION

In this section, we provide the explicit form of the driven-dissipative Gross-Pitaevskii equation (GPE) and the parameters used to obtain the numerical results presented in Sec. IV of the main manuscript. In the presence of a drive, dissipation, and exciton-exciton interactions, polaritons can be described using a two-component GPE of the form (see, e.g., [1])

$$i\hbar\partial_t \begin{pmatrix} \psi_{\rm X}(\mathbf{x}, t) \\ \psi_{\rm C}(\mathbf{x}, t) \end{pmatrix} = (H_0 + H_{\rm pot} + H_{\rm drive} + H_{\rm diss} + H_{\rm int}) \begin{pmatrix} \psi_{\rm X}(\mathbf{x}, t) \\ \psi_{\rm C}(\mathbf{x}, t) \end{pmatrix}, \tag{11}$$

where $\psi_{\rm X}(\mathbf{x}, t)$ and $\psi_{\rm C}(\mathbf{x}, t)$ are, respectively, the exciton and photon fields, and $H_0$, $H_{\rm pot}$, $H_{\rm drive}$, $H_{\rm diss}$ and $H_{\rm int}$ are Hamiltonian terms describing, respectively, the exciton-photon coupling (Eq. (1) of the main text), the exciton and

photon periodic potentials, the exciton and photon spectral linewidths, and the exciton-exciton interactions. More explicitly, the exciton-photon coupling is governed by

$$H_0 = \mathcal{F}^{-1} \begin{pmatrix} \omega^{\mathrm{X}}(\mathbf{q}) & g(\mathbf{q}) \\ g^*(\mathbf{q}) & \omega^{\mathrm{C}}(\mathbf{q}) \end{pmatrix} \mathcal{F}, \tag{12}$$

where $\omega^{\mathrm{X}}(\mathbf{q})$ and $\omega^{\mathrm{C}}(\mathbf{q})$ are, respectively, the exciton and photon energy dispersions, $g(\mathbf{q})$ is the exciton-photon coupling (Eq. (2) in the main text), and $\mathcal{F}$ denotes the Fourier transform defined such that $\mathcal{F}[\psi_{\mathrm{X,C}}(\mathbf{x}, t))] = \psi_{\mathrm{X,C}}(\mathbf{q}, t)$, where $\psi_{\mathrm{X}}(\mathbf{q}, t)$ and $\psi_{\mathrm{C}}(\mathbf{q}, t)$ are the momentum-space exciton and photon wavefunctions. The periodic exciton potential $V^{\mathrm{X}}(\mathbf{x})$ is introduced via

$$H_{\mathrm{pot}} = \begin{pmatrix} V^{\mathrm{X}}(\mathbf{x}) & 0 \\ 0 & 0 \end{pmatrix}. \tag{13}$$

The drive is described by

$$H_{\mathrm{drive}} = \begin{pmatrix} 0 & 0 \\ 0 & F_d(\mathbf{x}) e^{\mathrm{i}(\mathbf{k}_d - \omega_d t)} \end{pmatrix}, \tag{14}$$

where, $\mathbf{k}_d$ and $\omega_d$ are, respectively, the wave vector and the frequency of the drive, and $F_d$ is the spatial profile of the drive defined by the Gaussian function $F_d(\mathbf{x}) = f_d e^{-(\mathbf{x}-\mathbf{x}_d)^2/(2\sigma_d^2)}$, where $f_d$ is the amplitude of the drive and $\mathbf{x}_d$ and $\sigma_d$ are, respectively, the center position and the width of its spatial profile. Dissipation is captured in a phenomenological way using a non-Hermitian Hamiltonian term

$$H_{\mathrm{diss}} = \begin{pmatrix} -\mathrm{i}\gamma_{\mathrm{X}} & 0 \\ 0 & -\mathrm{i}\gamma_{\mathrm{C}} \end{pmatrix}, \tag{15}$$

where $2\gamma_{\mathrm{X}}$ and $2\gamma_{\mathrm{C}}$ are, respectively, the exciton and photon linewidths. Finally, exciton-exciton interactions are taken into account via

$$H_{\mathrm{int}} = \begin{pmatrix} g_{\mathrm{X}} |\psi(\mathbf{x}, t)|^2 & 0 \\ 0 & 0 \end{pmatrix}, \tag{16}$$

where $g_{\mathrm{X}}$ is the strength of the interactions. To produce the results presented in Fig. 7 of the main text, the above driven-dissipative GPE was solved numerically with (empty) initial conditions ($\psi_{\mathrm{X}}(\mathbf{x}, t_i) = 0$, $\psi_{\mathrm{C}}(\mathbf{x}, t_i) = 0$) at time $t_i = 0$, to a final time $t_f = 4 \cdot 10^3$ for a square system discretized on a spatial grid of $256 \times 256$ points. We use unitless parameters with the speed of light $v_C$ and the zero-momentum exciton energy $\omega^{\mathrm{X}}(\mathbf{0})$ set to unity. The remaining parameters take the form:

- system size: $80 \times 80$, with edges defined by a potential barrier of width 3 and height 5
- $\omega^{\mathrm{X}}(\mathbf{q}) = \omega^{\mathrm{X}}(\mathbf{0}) + q^2/(2m_{\mathrm{X}})$ with $\omega^{\mathrm{X}}(\mathbf{0}) = 1$ and $m_{\mathrm{X}} = 10^3$;
- $\omega^{\mathrm{C}}(\mathbf{q}) = v_{\mathrm{C}}|q|$ with $v_{\mathrm{C}} = 1$;
- $g(\mathbf{q}) = g_q e^{\mathrm{i}\theta(\mathbf{q})}$ with constant $g_q = 0.1$;
- $V^{\mathrm{X}}(\mathbf{x}) = V_{\mathrm{X}} \left(\cos(k_x x) + \cos(k_x x/2 + \sqrt{3} k_y y/2) + \cos(-k_x x/2 + \sqrt{3} k_y y/2)\right)$ with $V_{\mathrm{X}} = -0.05$ and $k_x = k_y = 1.88$ (corresponding to a lattice constant $a = 3.86$);
- $\mathbf{k}_d = \mathbf{0}$, $\omega_d = 0.856$, $f_d = 0.1$, $\mathbf{x}_d = (L_x/2, 1)$ ($(0, 0)$ being the position of the lower left corner of the system), $\sigma_d = 3$;
- $\gamma_{\mathrm{X}} = 5 \cdot 10^{-4}$, $\gamma_{\mathrm{C}} = 5 \cdot 10^{-4}$;
- $g_{\mathrm{X}} = 0.1$.

## III. SUPPLEMENTARY VIDEO

The supplementary video shows the time evolution of the intensity of the exciton and photon fields from $t_i = 0$ to $t_f = 4 \cdot 10^3$ with the same parameters as above.

---

[1] Carusotto, I. & Ciuti, C. Quantum fluids of light. *Rev. Mod. Phys.* **85**, 299–366 (2013).
